# Supplementary material for: Controlling the spin orientation of photoexcited electrons by symmetry breaking
Source: arXiv:1005.1280 ancillary file (2011-06-27)
Supplement: Supplementary file 1 [file supplementary_material.pdf]

# Auxiliary material to the paper "Controlling the spin direction of photoexcited electrons by symmetry breaking"

Lan Qing,* Yang Song, and Hanan Dery
*Department of Physics, University of Rochester, Rochester, New York, 14627*

**1. Numerical Tests.** We use a spin dependent pseudopotential model with 226 basis waves to test our effective mass description of conduction electrons with $s$-type symmetry. The spin-orbit interaction splits the two eigenstates in each band. Yet, photoexcited electrons generated from one valence band can be expressed as a coherent state of the conduction band eigenstates due to their small splitting and the finite spectral width of the exciting light. Fig. I shows the momentum and spin distributions of photoexcited hot electrons in GaAs. Apart from a minor warp along the $\langle 110\rangle$ plane, these 3D figures reinforce the used approximations.

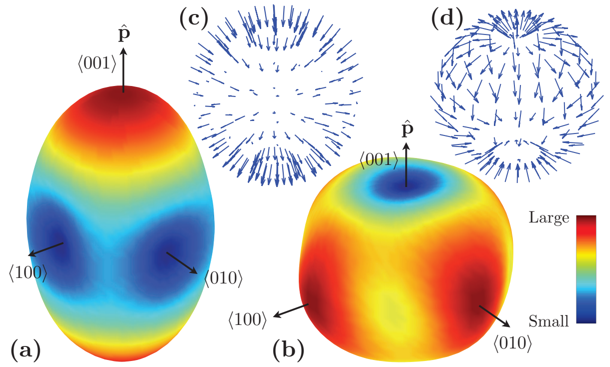


FIG. I: A pseduopotential model calculation of momentum alignment (a)-(b) and spin-momentum correlation (c)-(d) of photoexcited electrons that are generated with heavy holes (left) and light holes (right). The photons energy is 0.2 eV larger than the band-gap. The photons angular momentum is along the $\langle 001\rangle$ crystallographic axis.

**2. Monte Carlo Simulation.**

(a) Initial Wavevector and Spin. The electron's wavevector and spin immediately after photoexcitation is randomized according to the distributions in Eq. (1) of the main paper. The probability of exciting an electron by transition with a heavy hole is $[(m_{hh}/m_{lh})(m_e+m_{lh})/(m_e+m_{hh})]^{1.5}$ larger than with a light hole where $m_{e,hh,lh}$ are the effective mass of electrons, heavy holes and light holes, respectively. In GaAs, for example, the ratio is 2. In Simulations that neglect alignment and correlation the wavevector direction is uniformly randomized and the spin is along the light propagation axis.

(b) Initial Position. The initial position of the electron is randomized according to the light attenuation profile (exponential decay with photon penetration). The profile is calculated using material and photon energy dependent absorption coefficients from Ref. [*S1*].

(c) Transport. Transport in the bulk regions of the heterostructure follows the effective mass approximation.

(d) Spin Precession. The spin of an electron with wavevector $\mathbf{k}$ in the $\Gamma$-valley of zinc-blende semiconductor precesses about an intrinsic magnetic field with corresponding Larmor frequency components [*S2*], $\Omega_j(\mathbf{k}) = \alpha_c\hbar^2(2m_e^3E_g)^{-1/2}k_i(k_j^2-k_m^2)$ where $\{i,j,m\}$ denote any cyclic permutation of the crystallographic axes. $E_g$ is the band-gap and $\alpha_c$ is a dimensionless parameter related to the strength of the spin-orbit coupling ($\alpha_c = 0.07$ in GaAs [*S3*]). The spin evolution is denoted by,

$$\mathbf{S}(t) = \mathbf{S}_0\cos\Omega t + (\hat{\mathbf{\Omega}}\times\mathbf{S}_0)\sin\Omega t + (1-\cos\Omega t)(\hat{\mathbf{\Omega}}\cdot\mathbf{S}_0) \tag{I}$$

where $\mathbf{S}_0$ is the initial spin direction immediately after photoexcitation, reflection or scattering events. $\Omega$ and $\hat{\mathbf{\Omega}}$ are the magnitude and direction of the $\mathbf{\Omega}$ vector.

(e) Momentum and Energy Relaxation. Scattering times are randomized according to a homogeneous Poisson process, $\propto \exp\{-t/\tau(\varepsilon)\}$, where $\tau(\varepsilon)$ is an energy-dependent relaxation time constant. We assume low temperatures and consider relaxation of electrons by the Fröhlich interaction (via emission of longitudinal optical phonons). In polar semiconductors it is by far the dominant relaxation mechanism of hot electrons where [*S4*],

$$\frac{1}{\tau(\varepsilon)} = \frac{1}{\tau_0}\frac{3\zeta(k)}{4}\ln\left(\frac{1+\sqrt{1-\zeta^2(k)}}{1-\sqrt{1-\zeta^2(k)}}\right). \tag{II}$$

$\zeta(k) = \sqrt{\varepsilon_{LO}/\varepsilon(k)}$. The emitted phonon energy is $\varepsilon_{LO} = 36$ meV, and $\varepsilon(k) = \hbar^2k^2/2m_e$. The maximum rate appears at $\zeta = 0.55$ where $\tau(\varepsilon) = \tau_0$ (130 fs in GaAs [*S5*]). After scattering the electron changes its wavevector $\mathbf{k}\to\mathbf{k}'$ and its energy drops by $\varepsilon_{LO}$. The new wavevector ($\mathbf{k}'$) is randomized according to the favored forward scattering nature of the Fröhlich interaction, $|\mathbf{k}-\mathbf{k}'|^{-2}$ [*S4*]. The spin of the electron changes its wavevector dependent precession after scattering but it is not flipped by the scattering event (Elliott-Yafet mechanism is negligible during the initial energy relaxation).

(f) Complete reflection. When the electron reaches the interface, its wavevector component along the interface normal, $k_n = \mathbf{k}\cdot\hat{\mathbf{n}}$, flips sign and the electron changes its motion direction. Complete reflection is considered for wide barriers when tunneling is negligible and the energy of the electron is below the barrier edge.

(g) Partial reflection. Reflection or transmission of an electron across an interface is randomized according

to the values of the reflection coefficients. These values are calculated by numerical solutions of a simple 1D Schrödinger equation of the heterostructure. In case of partial reflection off a ferromagnet, the spin of a reflected electron can also change direction (ferromagnetic proximity effect). To simulate this effect we define the reflection matrix $\mathcal{R} = \frac{1}{2}[(r_\uparrow + r_\downarrow)\mathcal{I} + (r_\uparrow - r_\downarrow)\hat{\boldsymbol{\sigma}} \cdot \hat{\mathbf{m}}]$ where the spin-dependent reflection coefficient, $r_\uparrow$ ($r_\downarrow$), is associated with the majority (minority) spin direction $\hat{\mathbf{m}}$ ($-\hat{\mathbf{m}}$) of the reflecting material (the non-magnetic reflection is the case of $r_\uparrow = r_\downarrow$ and $\hat{\mathbf{m}} = 0$). The density matrix of the electron turns from $\mathcal{A}$ before reflection to $\mathcal{A}' = \mathcal{R}\mathcal{A}\mathcal{R}^\dagger$ after reflection, where $\mathcal{A} = [\mathcal{I} + \hat{\boldsymbol{\sigma}} \cdot \mathbf{S}]/2$ and $\mathbf{S}$ is the spin of the electron before reflection. The expectation value of the spin after reflection is obtained by taking traces $\mathbf{S}' = \mathrm{Tr}(\hat{\boldsymbol{\sigma}}\mathcal{A}')/\mathrm{Tr}(\mathcal{A}')$. The alignment, correlation and coherent precession play a crucial role since the tipping angle is acquired shortly after photoexcitation (see Fig. 2(d) of the main paper). The electron's wavevector direction which sets the magnitude of the reflection coefficients is still correlated with the spin direction at these timescales. These features determine the ferromagnetic imprinting signatures (see Fig. 3 of the main paper).

The simulation of all the above processes ends after $\sim$ 1 ps when the electron reach the conduction band bottom and the tipping process has effectively stopped. The spin relaxation at later times is $\sim 10^3$ slower ($k^3$-dependence of the precession frequency). The procedure is repeated for $N = 10^9$ particles. The information is thus stored in the net-spin vector (average of $N \gg 1$ electrons).

**3. Derivation of Eq (2) in the main paper.** From the shown time evolution in Fig. 2(d) of the main paper, we see that the precession induced tipping angle is accumulated shortly after excitation (and that accordingly $\Omega t < 1$). To derive analytical expressions we consider homogenous electron population between reflection barriers and we integrate over $k$-space using the distribution in Eq. (1) of the main paper. This procedure yields,

$$\mathbf{S}_\mathrm{f} = S_0\left[(1-\delta_a)\hat{\mathbf{p}} - \delta_b(\hat{\mathbf{p}}\cdot\hat{\mathbf{n}})\hat{\mathbf{n}}\right] , \qquad \text{(III)}$$

By considering a time distribution of $\propto \exp\{-t/\tau_{LO}\}$ for electrons before their first scattering events one gets,

$$\delta_{b,0} \approx \frac{\alpha_c^2\tau_{LO}^2}{\hbar^2 E_g}\gamma_{p,0}(\hbar\omega - E_g)^3 . \qquad \text{(IV)}$$

$$\gamma_{p,0} = \frac{32}{105 m_e^3}\sum_{i=1,2}\frac{r_i}{r_0}\frac{1}{1+e^{\xi_i}}\left[\frac{e^{\xi_i}-\xi_i-1}{\xi_i} + \frac{D_i}{1+e^{\xi_i}}\right] .$$

$$\xi_i = \frac{16\sqrt{2}L}{\tau_{LO}\left(A_i + B_i(\hat{\mathbf{p}}\cdot\hat{\mathbf{n}})^2\right)}\left[\frac{m_e^2}{m_i(\hbar\omega - E_g)}\right]^{\frac{1}{2}} ,$$

$r_0 = m_1^{\frac{3}{2}} + m_2^{\frac{3}{2}}$ where $m_{1,2}^{-1} = m_e^{-1} + m_{hh,lh}^{-1}$ and $r_i = m_i^{\frac{9}{2}}$. Other constants are $D_1 = 1.5$, $D_2 = 0.5 + 2e^{\xi_2}$, $A_1 = 15$, $A_2 = 17$, $B_1 = 3$ and $B_2 = -3$. After the first scattering the randomization in distribution leads to $A_i = 16$, $B_i = 0$ and $D_i = 1 + e^{\xi_i}$. Using the structure parameters of Fig. 2(a) of the main paper ($L = 50$ nm, $m_e = 0.067m_0$, $m_{hh} = 0.62m_0$ and $m_{lh} = 0.087m_0$) and also that $\hat{\mathbf{p}}\cdot\hat{\mathbf{n}} = 1/\sqrt{2}$ and $\tau_{LO} = 130$ fs, we get $\gamma_{p,0} \approx 0.06$ and $\gamma_{p,n>0} \approx 0.08$ where these values remain valid across a wide photon energy range, $\hbar\omega - E_g < 0.3$ eV.

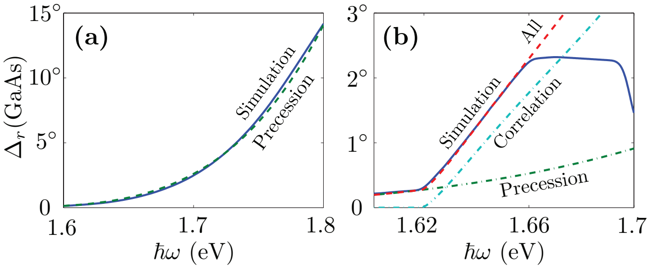


FIG. II: Simulated results and theoretical approximations (a) with setup (i) for precession induced tipping, and (b) with setup (ii) for both precession and correlation induced tipping.

Using Eq. (III) the tipping angel is $\Delta_p = \measuredangle\{\mathbf{S}_\mathrm{f}, \mathbf{S}_\mathrm{i}\}$ where $\mathbf{S}_\mathrm{i} = S_0\hat{\mathbf{p}}$ is the average initial spin. Thus,

$$\sin\Delta_p = \frac{\delta_b(\hat{\mathbf{p}}\cdot\hat{\mathbf{n}})\left[1-(\hat{\mathbf{p}}\cdot\hat{\mathbf{n}})^2\right]^{\frac{1}{2}}}{\left[(1-\delta_a)^2 + 2(1-\delta_a)\delta_b(\hat{\mathbf{p}}\cdot\hat{\mathbf{n}})^2 + \delta_b^2(\hat{\mathbf{p}}\cdot\hat{\mathbf{n}})^2\right]^{\frac{1}{2}}} .$$

Since $\delta_a$ and $\delta_b$ are small numbers one gets,

$$\Delta_p \approx \delta_b(\hat{\mathbf{p}}\cdot\hat{\mathbf{n}})\left[1-(\hat{\mathbf{p}}\cdot\hat{\mathbf{n}})^2\right]^{\frac{1}{2}} . \qquad \text{(V)}$$

In the optimal case ($\hat{\mathbf{p}}\cdot\hat{\mathbf{n}} = 1/\sqrt{2}$) we have $\Delta_p \approx \delta_b/2$ and the total accumulated angle after relaxation to the bottom of the conduction band is,

$$\Delta_p \approx \frac{\alpha_c^2\tau_{LO}^2}{2\hbar^2 E_g}\sum_{n=0}^{N}\gamma_{p,n}(\hbar\omega - E_g - nE_{LO})^3 , \qquad \text{(VI)}$$

where $N = \lfloor(\hbar\omega - E_g)/E_{LO}\rfloor$. Eq. (VI) is Eq. (2) of the main paper. Figure II(a) shows the agreement between this approximated expression (dash line) and the Monte Carlo simulation results (solid line; the same as the solid line in Fig. 2(c) of the main paper).

**4. Derivation of Eq (3) in the main paper.** We derive the tipping angle due to spin-momentum correlations of photoexcited electrons using a scheme of a step potential barrier. In the case of Fig. 2(a) of the main paper this scheme refers to the GaAs region and its $E_1$ potential step. To derive analytical expressions we consider homogenous electron population in the photoexcited region. We focus on a narrow photon energy region where the only electrons that can propagate to the barrier region are those that were generated by heavy-holes. In terms of Fig. 2(e) of the main paper, this case refers to photon energies below the first plateau

(1.62 eV $< \hbar\omega <$ 1.66 eV). Using this limiting case, the tipping angle is accumulated only prior to the first scattering event (after this scattering the total energy of an electron is below the potential step). After integration in $k$-space using the distribution in Eq. (1) of the main paper, and considering the partial transmission into a step barrier of height $E_B$, we get a similar expression to Eq. (III) where the correlation related $\delta_b$ parameter reads,

$$\delta_b = \frac{\beta_0}{S_0}\gamma_c\left[\vartheta^{3/2} - 1.5\vartheta^2 + 0.1\vartheta^{5/2} + \vartheta^3 + \mathcal{O}(\vartheta^{7/2})\right], \quad \text{(VII)}$$

$$\gamma_c \approx \frac{m_1^{3/2}}{m_1^{3/2} + m_2^{3/2}}\left[1 - \exp\left(-\frac{L}{\tau_{\rm LO}}\sqrt{\frac{2m_e}{E_B}}\right)\right]\frac{\tau_{\rm LO}}{L}\sqrt{\frac{E_B}{2m_e}},$$

where $\beta_0$ is the spin-momentum correlation parameter of photoexcited electrons generated via transitions with heavy holes. $\vartheta = [m_1(\hbar\omega - E_g)/(m_e E_1)] - 1$ and $m_{1,2}^{-1} = m_e^{-1} + m_{hh,lh}^{-1}$. Using these expressions one gets that in the optimal case ($\hat{\mathbf{p}} \cdot \hat{\mathbf{n}} = 1/\sqrt{2}$),

$$\Delta_c \approx \frac{\beta_0}{2S_0}\gamma_c\left(\vartheta^{3/2} - 1.5\vartheta^2 + 0.1\vartheta^{5/2} + \vartheta^3\right), \quad \text{(VIII)}$$

where $\gamma_c \approx 0.4$. Eq. (VIII) is Eq. (3) of the main paper ($E_B = E_1$). The dash line in Fig. II(b) denotes the sum of the approximated expressions of $\Delta_c$ and $\Delta_p$. The solid line denotes the Monte Carlo simulation (solid line; Fig. 2(e) of the main paper).

**5. Deriving Eq. (4) of the main paper.** We consider a non-ohmic tunneling barrier of width $d$ and height $E_B$ from the semiconductor conduction band. Spin selective reflection off a magnetic material originates from the difference in spin dependent wavevectors of its electrons, $k_\uparrow \neq k_\downarrow$ (Fermi wavevectors for majority and minority electrons in Fe are, respectively, 1.1 Å$^{-1}$ and 0.42 Å$^{-1}$ [*S7*]). The reflection coefficients of the barrier are given by [*S6*],

$$1 - |r_\uparrow|^2 = h_1 k_n e^{\chi_1 k_n^2}, \; 1 - |r_\downarrow|^2 = h_2 k_n e^{\chi_2 k_n^2}, \quad \text{(IX)}$$

$$1 - \text{Re}(r_\uparrow^* r_\downarrow) = h_0 k_n e^{\chi_0 k_n^2}, \; \text{Im}(r_\uparrow^* r_\downarrow) = h_3 k_n e^{\chi_3 k_n^2},$$

$$h_{1,2} = \tfrac{2G}{\kappa_0}\tfrac{\eta_{\uparrow,\downarrow}}{1+\eta_{\uparrow,\downarrow}^2}, \; h_0 = \tfrac{h_1+h_2}{2}, \; h_3 = \tfrac{\eta_\uparrow - \eta_\downarrow}{1+\eta_\uparrow\eta_\downarrow}h_0, \; \chi_i = \tfrac{c_i d}{\kappa_t}.$$

The electron's wavevector component along the interface normal in the semiconductor side, $k_n = \mathbf{k} \cdot \hat{\mathbf{n}}$, depends on whether the electron is generated with a heavy or a light hole. $\kappa_t = \sqrt{2m_e E_B}/\hbar$ denotes an effective tunneling wavevector, and $\eta_{\uparrow(\downarrow)} = (m_e/m_r)(k_{\uparrow(\downarrow)}/\kappa_0)$ denote spin-dependent velocity ratios. $m_e$ ($m_r$) is the effective mass in the semiconductor (reflecting material). $\kappa_0$, $c_i$ and $G$ depend on the barrier shape. In rectangular barriers $\kappa_0 = \kappa_t$, $G = 8e^{-2\kappa_t d}$, and $c_i = 1$. For parabolic Schottky barriers (homogeneously doped semiconductors) we use the confluent hypergeometric limit function [*S8*] and get $\kappa_0 = \frac{\kappa_t d}{3}\left[{}_0\mathrm{F}_1\left(;\tfrac{7}{4};\tfrac{\kappa_t^2 d^2}{16}\right)\Big/{}_0\mathrm{F}_1\left(;\tfrac{3}{4};\tfrac{\kappa_t^2 d^2}{16}\right)\right]$,

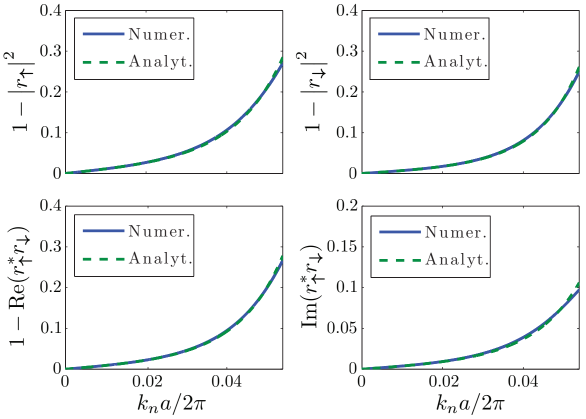


FIG. III: Numerical and analytical values of the reflection coefficients versus wavevector component along the interface normal. The calculations are made for a 0.5 eV high and 6 nm wide parabolic barrier. We use $c_0 = 3.11$, $c_1 = 2.78$, $c_2 = 3.48$, $c_3 = 2.93$. $a$=5.64 Å is the GaAs lattice constant.

$G = 2\Big/{}_0\mathrm{F}_1^2\left(;\tfrac{3}{4};\tfrac{\kappa_t^2 d^2}{16}\right)$ and $c_i$ are tedious dimensionless expressions of the order of unity (calculated by a Taylor series). Fig. III shows that using the analytical expressions in Eq. (IX) is an excellent approximation.

To get an approximated analytical expression for the net-spin after reflection off a ferromagnet, we substitute Eq. (IX) into $\mathcal{RDR}^\dagger$ where $\mathcal{D}$ is taken from Eq. (1) of the main paper and $\mathcal{R} = \frac{1}{2}[(r_\uparrow + r_\downarrow)\mathcal{I} + (r_\uparrow - r_\downarrow)\hat{\boldsymbol{\sigma}} \cdot \hat{\mathbf{m}}]$. The net-spin after reflection is given by,

$$\mathbf{S}_r = n_0 \ell S_0 \hat{\mathbf{p}} - \frac{\hbar\tau_\varepsilon}{8\pi^3 m_e}\int_{k_n>0} d^3k\, k_n \text{Tr}\left\{\frac{\hat{\boldsymbol{\sigma}}}{2}\left(\mathcal{D} - \mathcal{RDR}^\dagger\right)\right\},$$

where $\ell$ is the inverse of light absorption coefficient, $n_0$ is the density of excited electrons, and $\tau_\varepsilon$ is the relaxation time constant at the excitation energy (Eq. II). The analytical result of the integration is given by Eq. (4) of the main paper where the $\lambda_i$, $\delta_i^\alpha$ and $\delta_i^\beta$ parameters read,

$$\lambda_i = C_i \sum_{j=1,2} m_j^{3/2}(e^{x_{ij}} - y_{ij}), \quad \text{(X)}$$

$$\delta_i^{\mu=\alpha,\beta} = C_i \sum_{j=1,2} \frac{\mu(j) m_j^{3/2}}{x_{ij}}\{(\tfrac{9}{4} - x_{ij})e^{x_{ij}} - (\tfrac{9}{4} + \tfrac{1}{2}x_{ij})y_{ij}\}.$$

$j = 1$ ($j = 2$) corresponds to excitations with heavy (light) holes where $\mu(j) = (-1)^j$ and $m_{1,2}^{-1} = m_e^{-1} + m_{hh,lh}^{-1}$. Using $h_i$ & $\chi_i$ from Eq. (IX) one gets $C_i = \hbar\tau_\varepsilon h_i/\{16\chi_i m_e(m_1^{3/2} + m_2^{3/2})\}$, $x_{ij} = 2\chi_i m_j(\hbar\omega_0 - E_g)/\hbar^2$ and $y_{ij} = x_{ij}^{-1/2}\int_0^{\sqrt{x_{ij}}}\exp(w^2)dw$.

Finally, we mention that a number of ab-initio theoretical studies of ideal GaAs/Fe interfaces pointed out that the spin-down channel is blocked ($|r_\downarrow| = 1$) [*S9*, *S10*]. With this argument a larger signal is expected (increased values of $\lambda_1 - \lambda_2$ and $\delta_1^\alpha - \delta_2^\alpha$ in Eq. (4) of the main paper).

**6. Semiconductors with inversion symmetry.** Prolonged alignment and correlation signatures in semiconductors with inversion symmetry are possible by partial reflection. For example, in silicon the $\hat{\mathbf{k}}$ parameter in Eq. (1) of the main paper is replaced with $\mathbf{k}_0/k_0$ where $\mathbf{k}_0$ denotes any of the six wavevectors at the valley centers. In addition, the values of $\alpha$, $\beta$ and $S$ depend mainly on parameters of the dominant transverse-optical phonon assisted transition. The alignment and correlation signatures would only be effective by reflection of electrons from valleys whose $\mathbf{k}_0$ is perpendicular to the normal of the interface. The reason is that tunneling with the five times heavier longitudinal component is exponentially less effective [*S11*]. An intuitive effect is that for excitation by a linearly polarized light the ferromagnetic signature along $\hat{\mathbf{m}}$ is weaker if $|\hat{\mathbf{e}} \cdot \hat{\mathbf{n}}| = 1$ [*S12*].

**7. Possible Experiments.** In case of photoluminescence measurements, one should overcome the Snell's limitation that restricts the propagation angles inside the semiconductor to less than 20 degrees from the normal (e.g., in GaAs the refractive index is 3.5 and therefore the maximal angle for light propagation inside the semiconductor is $\sin^{-1}\theta = 1/3.5 \rightarrow \theta = 16.6°$). One possible solution to overcome this problem is to employ an index-matched hemispherical coupling lens that are in contact with the studied semiconductor (for example, index-matched hemisphere or Weierstrass coupling lens made of gallium phosphide on top of a GaAs slab). This will allow the light (excited and emitted) to propagate inside the semiconductor at large angles with respect to the normal of the semiconductor sample.

Another possible experiment relates to the nuclear spin system. Straight detection of precession and correlation induced mechanisms via NMR would be difficult. However, detecting nuclear polarization via the Overhauser effect with a time resolved electron spin precession experiment [*S13*, *S14*] may be a good approach to study the correlation, alignment and coherent precession of photoexcited hot electrons (say 0.1-0.3 eV above the conduction band edge). The idea would be that the tipping mechanisms would tip electron spins in or out of the direction of an applied magnetic field. As a result, the buildup of nuclear polarization would cause enhanced or suppressed electron precession frequencies. In this setup, the tipping angle can be measured with extremely high precision via the precession frequency changes (so that even very small influence of tipping can be detected).

Without the tipping mechanisms, dynamical nuclear polarization measurements are not efficient in studying the spin-orbit coupling parameters of **hot** electrons due to their highly delocalized nature. For example, at low temperatures in **bulk** GaAs localized electrons (bound to impurities) or electrons that are at the very bottom of the conduction band can polarize the nuclear system several orders of magnitude faster than in case of highly delocalized electrons that reside 0.2 eV above the conduction band edge (see, e.g., section 9 in Ref. [*S15*]). On the other hand, after relaxation to the bottom of the conduction band, the tipped net-spin vector (induced by symmetry breaking) can polarize the nuclear system. When 'cold' electrons are trapped (localized) on donor impurities the polarization of the nuclear spin system becomes much more effective and the tipping angle can be used to extract spin-orbit coupling parameters from the ultrashort phase during which the electron were hot.

Finally, the tipping angle can also be used to extract parameters on the exciting conditions. For example, one can infer the crystal axes from the tipping angle or the incident beam propagation direction or the photon energy (if a small device footprint is required at the expense of energy resolution). All of these detection possibilities can rely on the tipping angles and they are insensitive to the intensity of the incident light beam (no need to know or compensate for surface roughness, spurious reflections and previous loss of the optical signal).

* Electronic address: lan.qing@rochester.edu

[S1] B. Monemar, K. K. Shih, and G. D.Pettit, J. Appl. Phys. **47**, 2604 (1976).
[S2] M. I. Dyakonov, V. I. Perel, Sov. Phys. JETP **33**, 1053 (1971); Sov. Phys. Solid State **13**, 3023 (1972).
[S3] V. A. Marushchak, M. N. Stepanova, and A. N. Titkov, Sov. Phys. Solid State **25**, 2035 (1983).
[S4] M. Lundstrom, *Fundamentals of Carrier Transport* (Cambridge University Press, Cambridge, 2000), Ch. 2.
[S5] E. M. Conwell and M. O. Vassel, IEEE Trans. Electron Devices **12**, 22 (1966).
[S6] Y. Song and H. Dery, Phys. Rev. B **81**, 045321 (2010).
[S7] J. C. Slonczewski, Phys. Rev. B **39**, 6995 (1989).
[S8] Defined in *Mathematica* as Hypergeometric0F1[b, z].
[S9] J. M. MacLaren, X.-G. Zhang, W. H. Butler, and X. Wang, Phys. Rev. B **59**, 5470 (1999).
[S10] O.Wunnicke, Ph. Mavropoulos, R. Zeller, P.H. Dederichs, and D. Grundler *et al.*, Phys. Rev. B **65**, 241306 (2002).
[S11] P. Mavropoulos, Phys. Rev. B **78**, 054446 (2008).
[S12] This is a result of preferential excitation in valleys along the light polarization vector. See, e.g., A. V. Efanov and M. V. Entin, Phys. Stat. Sol. (B) **118**, 63 (1983).
[S13] G. Salis, D. T. Fuchs, J. M. Kikkawa, D. D. Awschalom, Y. Ohno, and H. Ohno, Phys. Rev. Lett. **86**, 2677 (2001).
[S14] J. Kikkawa and D. D. Awschalom, Science **287**, 473 (2000).
[S15] M. I. Dyakonov and V. I. Perel, in *Optical Orientation*, edited by F. Meier and B. P. Zakharchenya, (North-Holland, New York, 1984), Ch. 2.
